# Supplementary material for: Isovolumetric dividing active matter
Source: arXiv:2409.20481 ancillary file (2024-09-30)
Supplement: Supplementary file 1 [file supplement.pdf]

# Supplemental Material for "Isovolumetric dividing active matter"

Samantha R. Lish,[1,2,*] Lukas Hupe,[1,3,*] Ramin Golestanian,[1,2,3] and Philip Bittihn[1,3,†]

[1] *Max Planck Institute for Dynamics and Self-Organization, Göttingen, Germany*

[2] *Rudolf Peierls Centre for Theoretical Physics, University of Oxford, Oxford OX1 3PU, United Kingdom*

[3] *Institute for the Dynamics of Complex Systems, Göttingen University, Göttingen, Germany*

## I. VOLUME-CONSERVING DIVISION

As described in the main text in Appendix A and Ref. [45], cells are approximated as soft binodal dumbbells, consisting of two 2D disks with initial radius, $R_0$, and reducing radius, $R(\gamma)$, expressed as a function of the growth progress $\gamma \in [0, 1)$, which can be thought of as an internal clock parameterizing the cellular life cycle. Without loss of generality, nodal positions are designated + and − (right and left, respectively, in Supp. Fig. S1). Elongation begins with two fully overlapping nodes at $\gamma = 0$ in the center of a disk cell ("Mother" in Supp. Fig. S1). As $\gamma$ increases towards 1, the nodes have a $\gamma$ and radius dependent preferred separation, modeled by a "backbone" spring of rest length $l(\gamma) = 2R(\gamma)\gamma$, resulting in dumbbell shapes during the intermediate period of elongation ("Binodal Elongation" in Supp. Fig. S1). Our aim is to determine the functional dependency $R(\gamma)$, such that the volume of the intermediate dumbbell shape is kept constant at the initial volume $\pi R_0^2$ for all $\gamma$. We assume that the backbone is at its rest length (i.e., the dumbbell has its nominal volume).

During elongation, the dumbbell area can be calculated by subtracting the area of disk overlap, $A_{\text{overlap}}(\gamma)$, from the total area of both disks, such that $A_{\text{dumbbell}}(\gamma) = 2\pi R^2(\gamma) - A_{\text{overlap}}(\gamma)$. The overlap $A_{\text{overlap}}(\gamma)$ consists of two circular sectors of area $\theta R^2$ without their inner triangular parts, where $\theta$ is half the opening angle as shown in Supp. Fig. S1. The inner triangular part of each sector has a height $l(\gamma)/2 = R(\gamma)\gamma$ and base $2\sqrt{R^2(\gamma) - (l(\gamma)/2)^2} = 2R(\gamma)\sqrt{1-\gamma^2}$ such that the overlap area evaluates to

$$A_{\text{overlap}}(\gamma) = 2\left[\theta R^2(\gamma) - R(\gamma)\gamma \cdot R(\gamma)\sqrt{1-\gamma^2}\right] \tag{1}$$

Noticing that $\cos(\theta) = [l(\gamma)/2]/R(\gamma) = \gamma$, we therefore have

$$A_{\text{dumbbell}}(\gamma) = 2\pi R^2(\gamma) - 2\left[\arccos(\gamma)R(\gamma)^2 - R^2(\gamma)\gamma\sqrt{1-\gamma^2}\right] \tag{2}$$

$$= 2R^2(\gamma)\left[\pi - \arccos(\gamma) + \gamma\sqrt{1-\gamma^2}\right]. \tag{3}$$

To solve for the reducing radius R($\gamma$) which would yield exact area conservation, we then

* these authors contributed equally
† philip.bittihn@ds.mpg.de

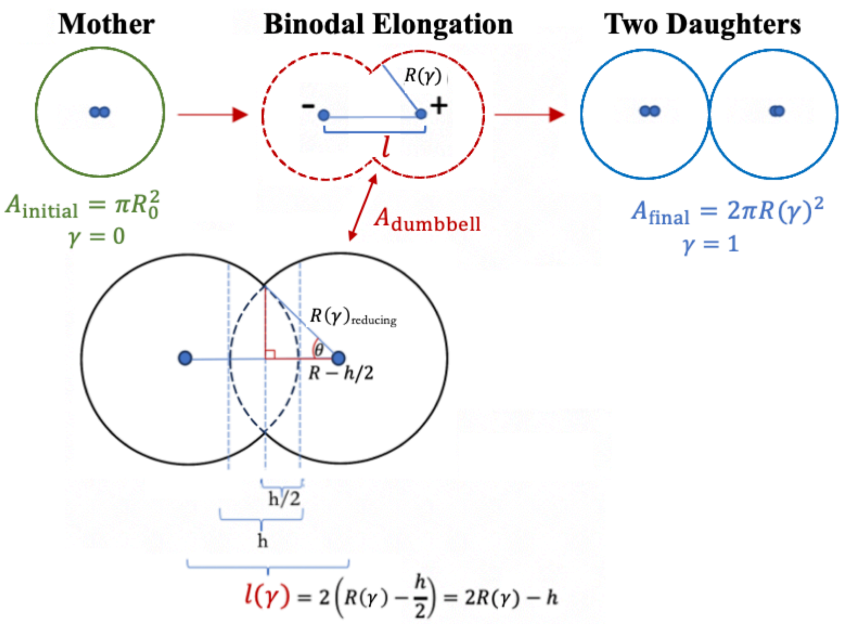


Supp. Fig. S1. **Shape changes accompanying growth and division.** Radius $R(\gamma)$ for interpolation between initial Mother and final Two Daughters is derived by requiring that the cell area $A_{\text{initial}} = A_{\text{dumbbell}}(\gamma) = A_{\text{final}}$ for all $\gamma \in [0, 1)$. All quantities are expressed in terms of time-dependent growth progress $\gamma$, which functions as an internal clock. At $\gamma = 1$, the dumbbell backbone length, $l(\gamma, R)$, reaches its maximum and the cell is divided into two equally sized daughter cells, each initialized with $\gamma = 0$.

set $A_{\text{dumbbell}}(\gamma) = \pi R_0^2$, yielding

$$R(\gamma) = R_0 \sqrt{\frac{\pi}{2\left[\pi - \arccos(\gamma) + \gamma\sqrt{1-\gamma^2}\right]}} \tag{4}$$

In simulation, daughter cells inherit the final reduced radius of their mother, $R_0/\sqrt{2}$, which ensures overall area conservation during successive embryonic cleavage divisions.

## II. PHYSICAL CIRCULAR CONTAINER

We repeated the full set of simulations from the main text with a physical circular boundary instead of periodic domain boundaries. Using the same initial cell size $R_0$, we used the same set of division rate distributions and volume fractions $\mathfrak{C}$. The latter was achieved by adjusting the domain radius $R_{\mathrm{domain}}$ such that $\mathfrak{C} = (R_0/R_{\mathrm{domain}})^2$ yields the desired values. The results are shown in Supp. Figs. S2 to S4,

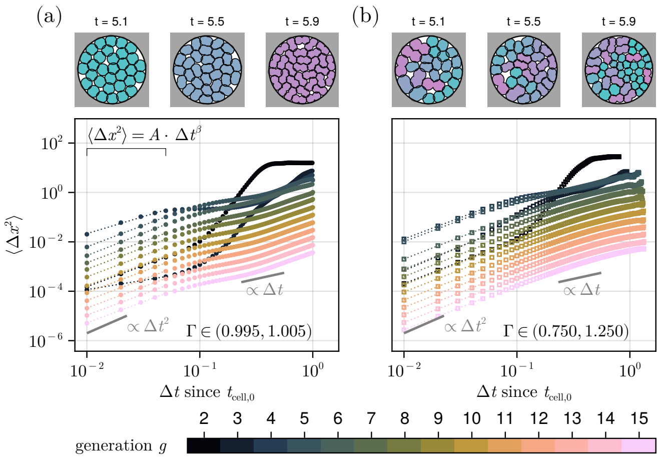


Supp. Fig. S2. Mean-squared displacements for cell centers by generation. Analogous to Main Figs. 1d and 1e, but for a physical circular boundary. (a) Narrow division rate distribution $\Gamma \in (0.995, 1.005)$. (b) Wide division rate distribution $\Gamma \in (0.75, 1.25)$.

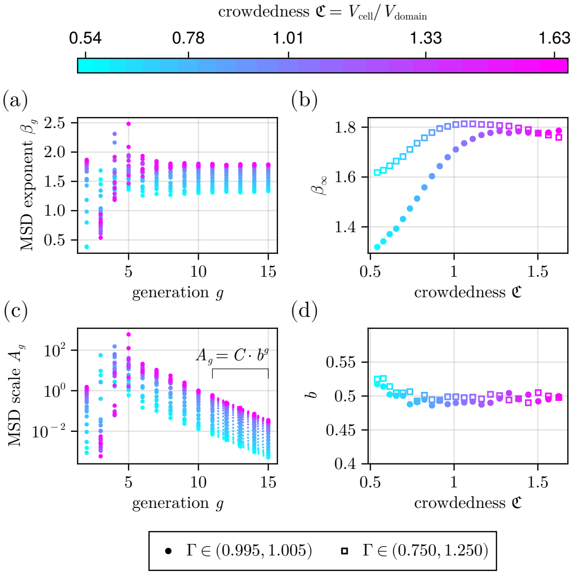


Supp. Fig. S3. Analysis of by-generation cell-center MSDs analogous to Main Fig. 2, but for a physical circular boundary, i.e. based on the data in Supp. Fig. S2.

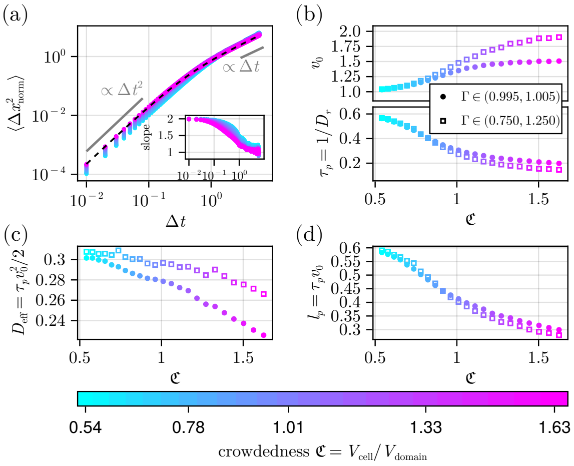


Supp. Fig. S4. Transgenerational compartment-based MSDs analogous to Main Fig. 2 panels c to f, but for a physical circular boundary.
